# Supplementary material for: Near-Online Multi-target Tracking with Aggregated Local Flow Descriptor
Source: arXiv:1504.02340 source file (2015-04-09)
Supplement: Supplementary file 1 [file appendix.tex]

\section{Some Appendix}
The contents...

\section{Some Appendix 2}
what?
